# Supplementary material for: Reynolds Number and Intermittency in the Expanding Solar Wind: Predictions Based on Voyager Observations
Source: arXiv:1905.02903 source file (2019-05-08)
Supplement: Supplementary file 1 [file Supplemental_Material.pdf]

**Reynolds Number and Intermittency in the Expanding Solar Wind: Predictions Based on Voyager Observations**

T. N. Parashar, M. Cuesta, W. H. Matthaeus
*Bartol Research Institute, Department of Physics and Astronomy, University of Delaware, Newark, DE*

**SUPPLEMENTAL MATERIAL**

The attached figure shows an example of possible “wave activity” that destroys coherence in the turbulent signal. Top panel shows the magnetic time series for the bin between 8.16-8.18AU. The insert shows a zoom in of BT in the region marked by red in the main panel. Within the insert, the red curve shows a 20 point (38.4s) running average of BT. Wave activity reminiscent of the upstream waves frequently observed [e.g. Smith et. al. JGR 1983] can be seen. Lower panels show the autocorrelation function (Cr), second order structure function $S^{(2)}$ and scale dependent kurtosis.

All the quantities show oscillations at various scales, especially the oscillations in kurtosis of BT at ~ 1000s are consistent with the ~1000s oscillation seen in the insert.

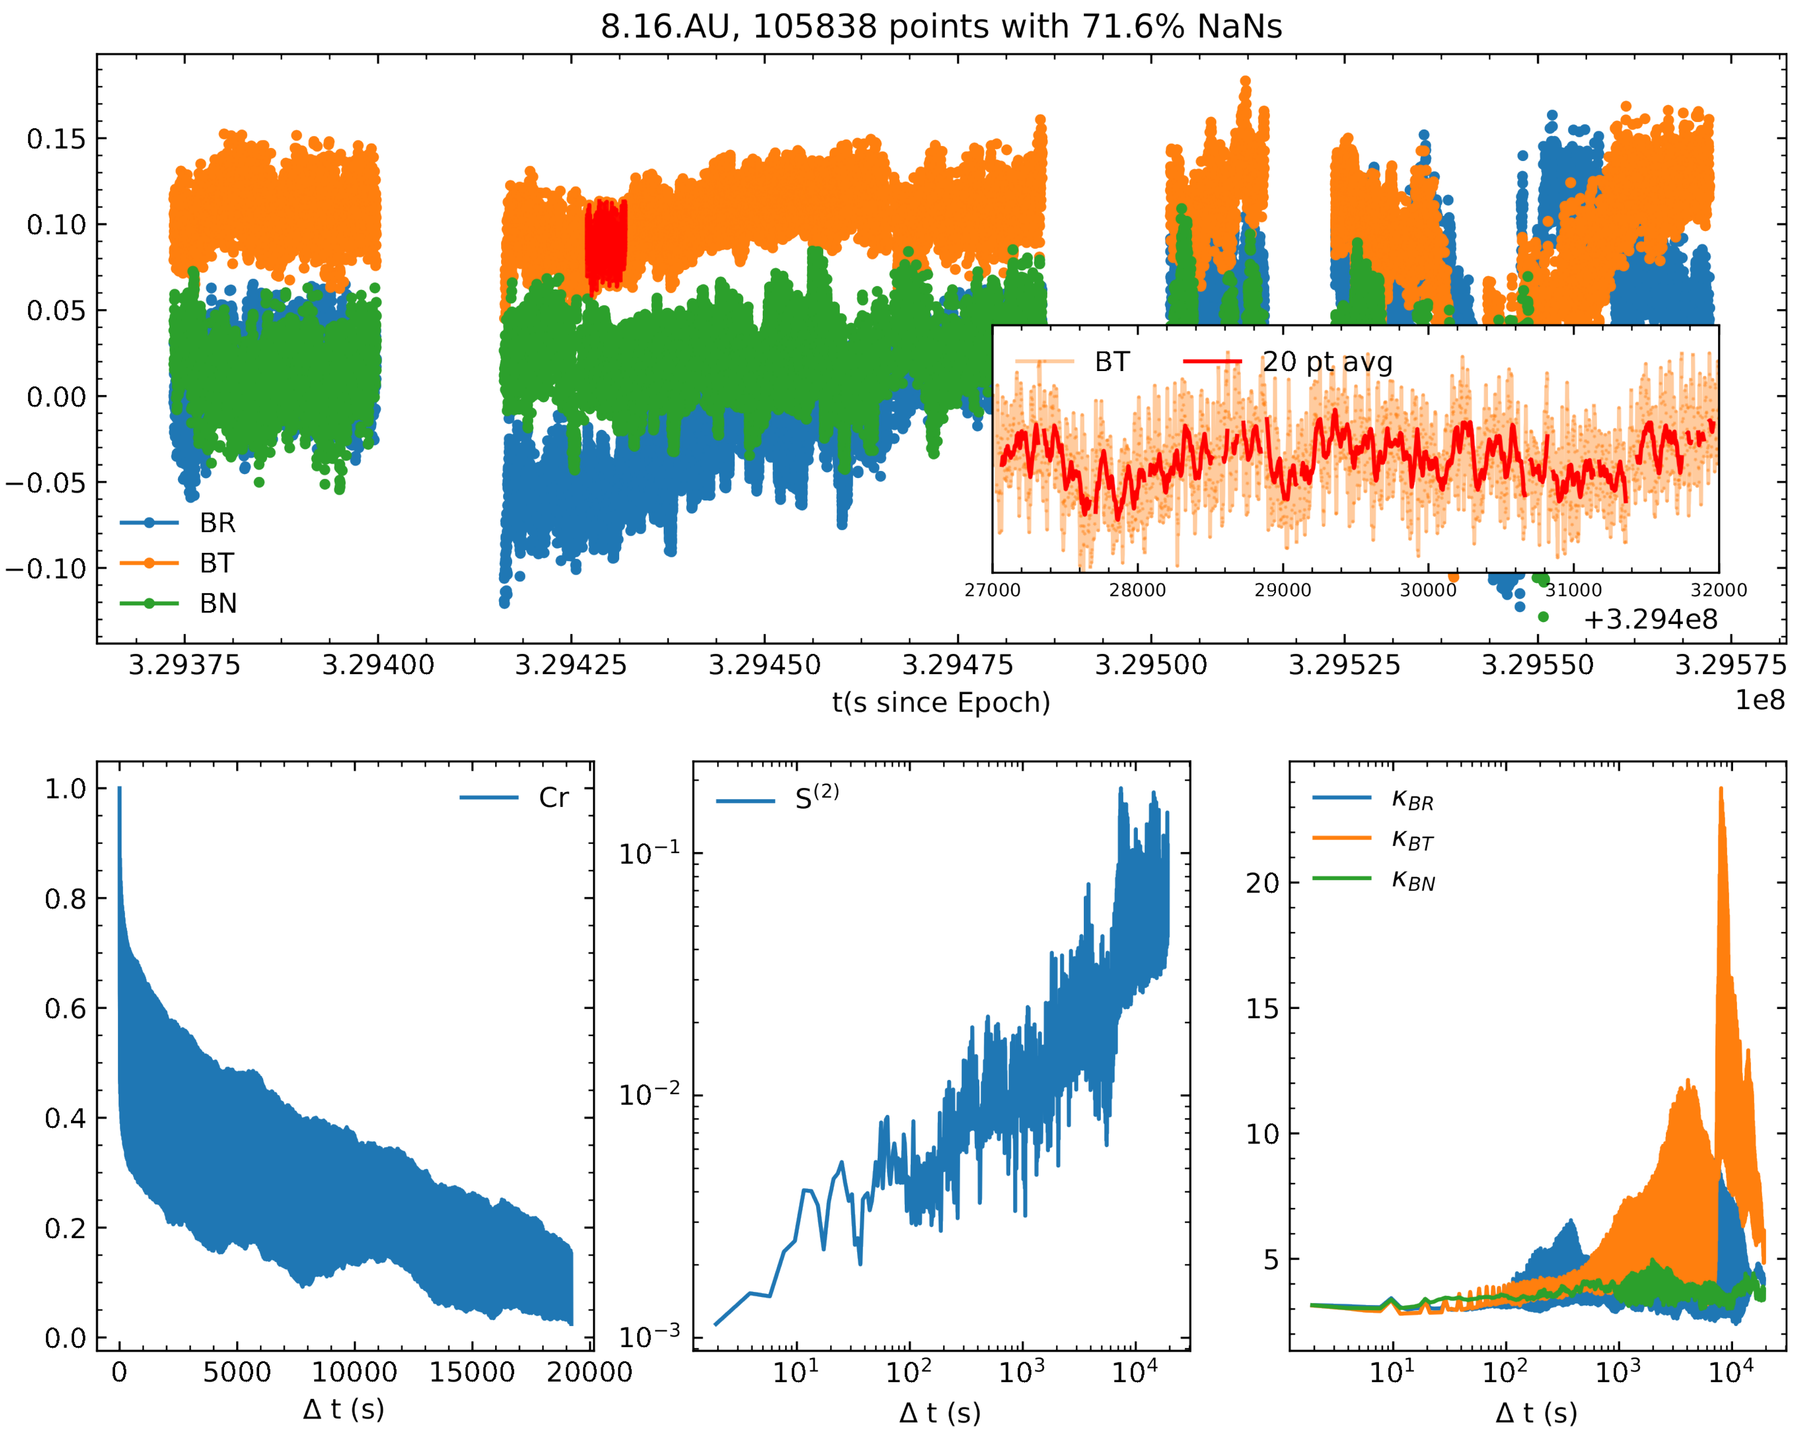

8.16.AU, 105838 points with 71.6% NaNs
BR
BT
BN
BT
20 pt avg
+3.294e8
t(s since Epoch)
1e8
Cr
$S^{(2)}$
$\kappa_{BR}$
$\kappa_{BT}$
$\kappa_{BN}$
Δ t (s)
Δ t (s)
Δ t (s)
